# Supplementary material for: Diversity of Radial Spin Textures in Chiral Materials
Source: arXiv:2304.11650 ancillary file (2023-04-23)
Supplement: Supplementary file 1 [file SM.pdf]

# Supplemental Material for:
# "Diversity of Radial Spin Textures in Chiral Materials"

Daniel Gosálbez-Martínez,[1, 2, 3, *] Alberto Crepaldi,[4] and Oleg V. Yazyev[2, 3, †]

[1]*Departamento de Física Aplicada, Universidad de Alicante, 03690 Alicante, Spain*
[2]*Institute of Physics, Ecole Polytechnique Fédérale de Lausanne (EPFL), CH-1015 Lausanne, Switzerland*
[3]*National Centre for Computational Design and Discovery of Novel Materials MARVEL, Ecole Polytechnique Fédérale de Lausanne (EPFL), CH-1015 Lausanne, Switzerland*
[4]*Dipartimento di Fisica, Politecnico di Milano, Piazza Leonardo da Vinci 32, Milan 20133, Italy*

## I. HIGH-SYMMETRY POINTS OF 45 NON-POLAR CHIRAL SPACE GROUPS

TABLE I: Complete list of high-symmetry points of 45 non-polar chiral space groups. Their point groups and time-reversal invariance are given.

| Space group | High-symmetry point | Point group | TRIM |
|---|---|---|---|
| 16 ($P222$) | Γ,Y, X, Z, U, T, S, R | $D_2$ | yes |
| 17 ($P222_1$) | Γ,Y, X, S | $D_2$ | yes |
| 18 ($P2_12_12$) | Γ, Z | $D_2$ | yes |
| 19 ($P2_12_12_1$) | Γ | $D_2$ | yes |
| 20 ($C222_1$) | Γ, Y | $D_2$ | yes |
| 21 ($C222$) | Γ,Y, Z, T | $D_2$ | yes |
| 22 ($F222$) | Γ,Y, X, Z | $D_2$ | yes |
| 23 ($I222$) | Γ, X | $D_2$ | yes |
| | W | $D_2$ | no |
| 24 ($I2_12_12_1$) | Γ, X | $D_2$ | yes |
| | W | $D_2$ | no |
| 89 ($P422$) | Γ, M, Z, A | $D_4$ | yes |
| | R, X | $D_2$ | yes |
| 90 ($P42_12$) | Γ, Z | $D_4$ | yes |
| 91 ($P4_122$) | Γ, M | $D_4$ | yes |
| | X | $D_2$ | yes |
| 92 ($P4_12_12$) | Γ | $D_4$ | yes |
| 93 ($P4_222$) | Γ, M, Z, A | $D_4$ | yes |
| | R, X | $D_2$ | yes |
| 94 ($P4_22_12$) | Γ, Z | $D_4$ | yes |
| 95 ($P4_322$) | Γ, M | $D_4$ | yes |
| | X | $D_2$ | yes |
| 96 ($P4_32_12$) | Γ | $D_4$ | yes |
| 97 ($I422$) | Γ, Z | $D_4$ | yes |
| | X | $D_2(C_{2b})$ | yes |
| | P | $D_2$ | no |
| 98 ($I4_122$) | Γ, Z | $D_4$ | yes |
| | X | $D_2(C_{2b})$ | yes |
| | P | $D_2$ | no |
| 149 ($P312$) | Γ, A | $D_3$ | yes |
| 150 ($P321$) | Γ, A | $D_3$ | yes |
| | K, H | $D_3$ | no |
| 151 ($P3_112$) | Γ, A | $D_3$ | yes |
| 152 ($P3_121$) | Γ, A | $D_3$ | yes |
| | K, H | $D_3$ | no |

* daniel.gosalbez@ua.es
† oleg.yazyev@epfl.ch

TABLE I (continued from previous page)

| Space group | High-symmetry point | Point group | TRIM |
|---|---|---|---|
| 153 ($P3_212$) | Γ, A | $D_3$ | yes |
| 154 ($P3_221$) | Γ, A | $D_3$ | yes |
| | K, H | $D_3$ | no |
| 155 ($R32$) | Γ, Z | $D_3$ | yes |
| 177 ($P622$) | Γ, A | $D_6$ | yes |
| | M, L | $D_2(C''_{21})$ | yes |
| | K, H | $D_3$ | no |
| 178 ($P6_122$) | Γ | $D_6$ | yes |
| | M | $D_2(C''_{21})$ | yes |
| | K | $D_3$ | no |
| 179 ($P6_522$) | Γ | $D_6$ | yes |
| | M | $D_2(C''_{21})$ | yes |
| | K | $D_3$ | no |
| 180 ($P6_222$) | Γ, A | $D_6$ | yes |
| | M, L | $D_2(C''_{21})$ | yes |
| | K, H | $D_3$ | no |
| 181 ($P6_422$) | Γ, A | $D_6$ | yes |
| | M, L | $D_2(C''_{21})$ | yes |
| | K, H | $D_3$ | no |
| 182 ($P6_322$) | Γ | $D_6$ | yes |
| | M | $D_2(C''_{21})$ | yes |
| | K | $D_3$ | no |
| 195 ($P23$) | Γ, R | $T$ | yes |
| | X, M | $D_2$ | yes |
| 196 ($F23$) | Γ | $T$ | yes |
| | X | $D_2$ | yes |
| 197 ($I23$) | Γ, H | $T$ | yes |
| | P | $T$ | no |
| 198 ($P2_13$) | Γ | $T$ | yes |
| 199 ($I2_13$) | Γ, H | $T$ | yes |
| | P | $T$ | no |
| 207 ($P432$) | Γ, R | $O$ | yes |
| | X, M | $D_4$ | yes |
| 208 ($P4_232$) | Γ, R | $O$ | yes |
| | X, M | $D_4$ | yes |
| 209 ($F432$) | Γ | $O$ | yes |
| | X | $D_4$ | yes |
| | L | $D_3(C^+_{31})$ | yes |
| | W | $D_2$ | yes |
| 210 ($F4_132$) | Γ | $O$ | yes |
| | X | $D_4$ | yes |
| | L | $D_3(C^+_{31})$ | yes |
| | W | $D_2$ | yes |
| 211 ($I432$) | Γ, H | $O$ | yes |
| | P | $T$ | no |
| | N | $D_2(C_{2b})$ | yes |
| 212 ($P4_332$) | Γ | $O$ | yes |
| 213 ($P4_132$) | Γ | $O$ | yes |
| 214 ($I4_132$) | Γ, H | $O$ | yes |
| | P | $T$ | no |
| | N | $D_2(C_{2b})$ | yes |

## II. COMPUTATIONAL METHODOLOGY

The electronic structure calculations have been performed within the density functional theory formalism using the planewave pseudopotentials method, as implemented in the `pwscf` code of the Quantum ESPRESSO package [1]. The exchange and correlation potentials were treated within the Perdew–Burke–Ernzerhof generalized gradient approximation [2]. Fully relativistic pseudopotentials were considered to include the spin-orbit coupling. For all elements we employed the ultrasoft pseudopotentials obtained from the PS library [3], with the only exception of cobalt for which a norm-conserving pseudopotential from the SG15 ONCV potentials database [4, 5] was used.

We performed self-consistent calculations of the ground state using the reported experimental values for the lattice parameters and atomic positions of the investigated materials. The crystal structures of $CoTeMoO_6$, $Ni_3S_2$, $TaSi_2$, CoSi and $Ag_3AuTe_2$ were obtained from the Crystallographic Open Database (COD) [6–8], while the structure of $Ta_2Se_8I$ was obtained from ICSD database [9]. The input files for all calculations were created using the `CIF2cell` code [10]. We used the Marzari-Vanderbilt-De Vita-Payne cold smearing [11] with a spread of 0.01 Ry. The sizes of the Monkhorst-Pack grid and the energy cutoffs for the planewave expansion are provided in Table II.

The spin textures were computed using the `bands` code of the Quantum ESPRESSO package [1]. The calculations were performed on a sphere of radius $0.005 \cdot 2\pi/a$ surrounding each high-symmetry point. We discretized the sphere with a uniform grid of points in spherical coordinates at an interval of $10^\circ$ in both polar $\theta$ and azimuthal $\phi$ coordinates.

TABLE II. Summary of materials examples for each type of spin texture

| Material | Monkhorst–Pack mesh | Planewave cutoff (Ry) |
|---|---|---|
| $CoTeMoO_6$ | $6 \times 6 \times 4$ | 80 |
| $Ni_3S_2$ | $8 \times 8 \times 8$ | 55 |
| $Ta_2Se_8I$ | $8 \times 8 \times 8$ | 60 |
| $TaSi_2$ | $9 \times 9 \times 7$ | 50 |
| CoSi | $6 \times 6 \times 6$ | 80 |
| $Ag_3AuTe_2$ | $6 \times 6 \times 6$ | 55 |

## III. ELECTRONIC STRUCTURE OF SELECTED MATERIALS

In this section, we provide details of the electronic structure of the selected materials to illustrate the radial spin texture. For each material we provide two figures. The first figure shows the unit cell, the corresponding Brillouin zone and the band structure along the high-symmetry points of the Brillouin zone. The second figure show the detailed view of the energy dispersion along high-symmetry directions for each band (shown in green) used to illustrate the radial spin textures in the main text. Additionally, we have illustrated the size of sphere for each high-symmetry direction with vertical red lines. The region shaded in red is the interior of the spheres of radius $0.005 \cdot 2\pi/a$.

### *1.* $CoTeMoO_6$

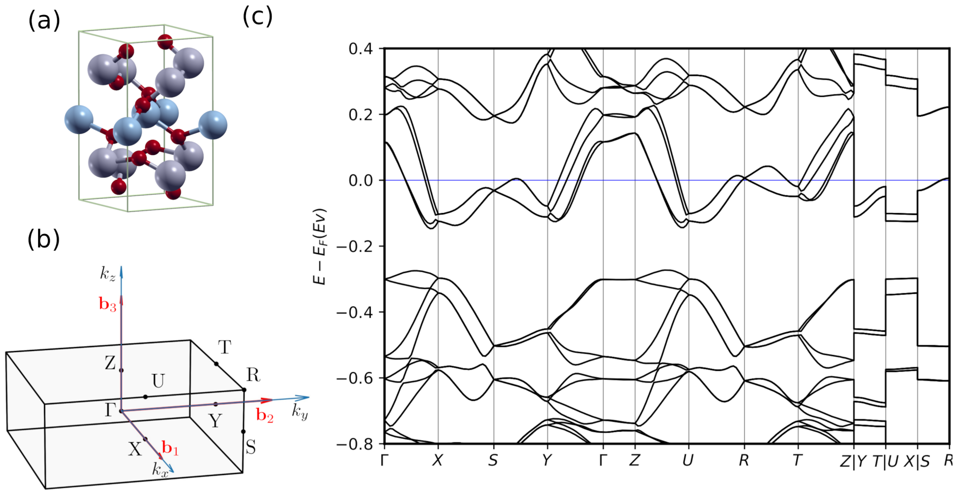


FIG. 1. (a) Crystal structure, (b) Brillouin zone with the high-symmetry points and reciprocal lattice vectors indicated, and (c) the calculated band structure of $CoTeMoO_6$ plotted along the high-symmetry lines.

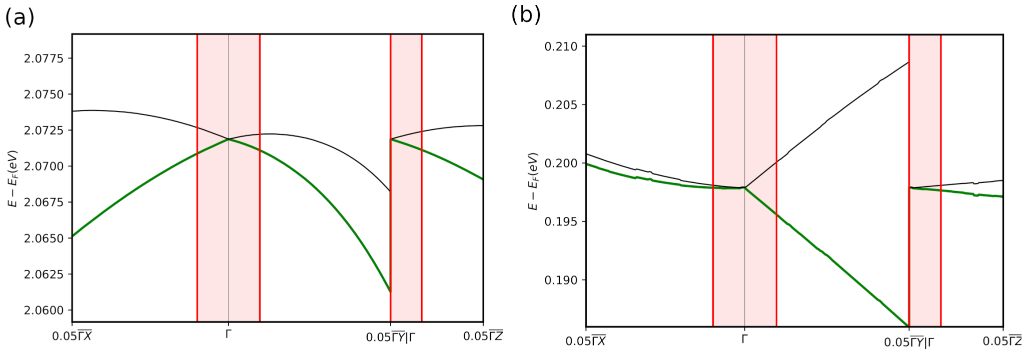


FIG. 2. Electronic band dispersion near the high-symmetry points of the selected bands to illustrate the spin texture of $CoTeMoO_6$. Vertical red lines illustrate the radius of the sphere along the corresponding high-symmetry direction. Panel (a) shows band $n = 156$ (in green) which correspond to the example of spin textures with linear momentum dependence illustrated in Fig. 1(f) of the main text. Panel (b) shows band $n = 146$ which correspond to the spin textures with cubic momentum dependence illustrated in Fig. 3(a) of the main text.

## 2. $Ni_3S_2$

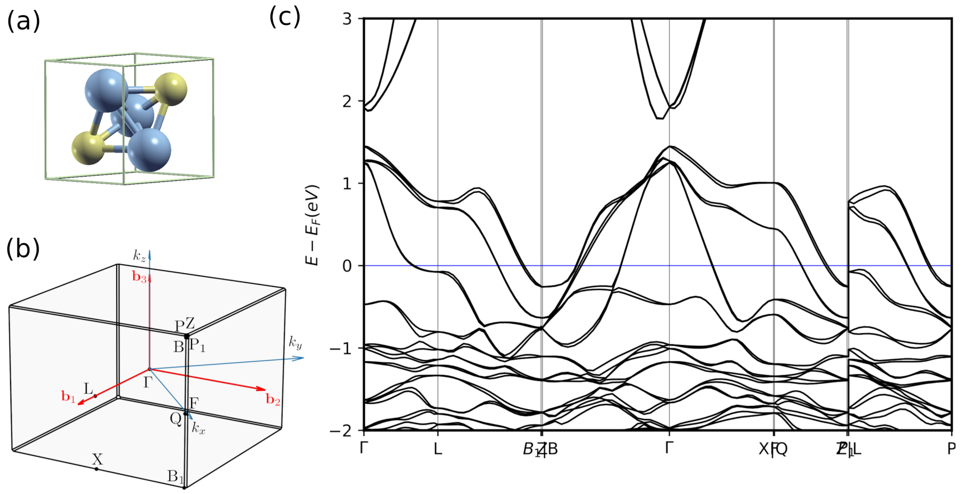


FIG. 3. (a) Crystal structure, (b) Brillouin zone with the high-symmetry points and reciprocal lattice vectors indicated, and (c) the calculated band structure of $Ni_3S_2$ plotted along the high-symmetry lines.

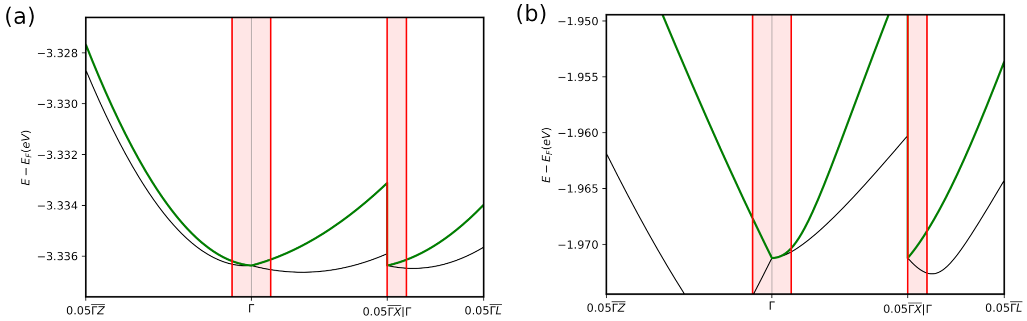


FIG. 4. Electronic band dispersion near the high-symmetry points of the selected bands used to illustrate the spin texture of $Ni_3S_2$. Vertical red lines delimit the radius of the sphere along the corresponding high-symmetry direction. Panel (a) shows band $n = 17$ (in green) which corresponds to the spin texture with linear momentum dependence illustrated in Fig. 1(c) of the main text. Panel (b) shows band $n = 27$ used to compute the spin texture with cubic momentum dependence illustrated in Fig. 3(b) of the main text.

### *3.* $Ta_2Se_8I$

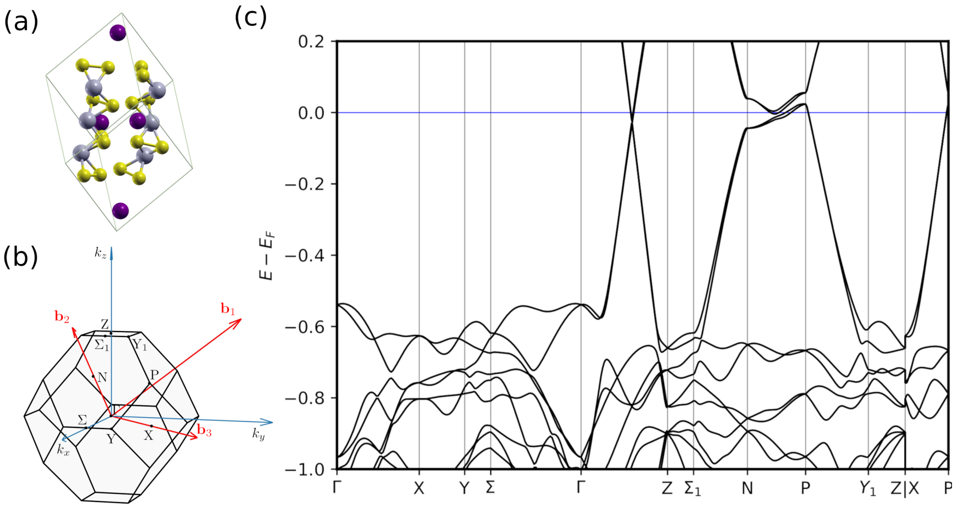


FIG. 5. (a) Crystal structure, (b) Brillouin zone with the high-symmetry points and reciprocal lattice vectors indicated, and (c) the calculated band structure of $Ta_2Se_8I$ plotted along the high-symmetry lines.

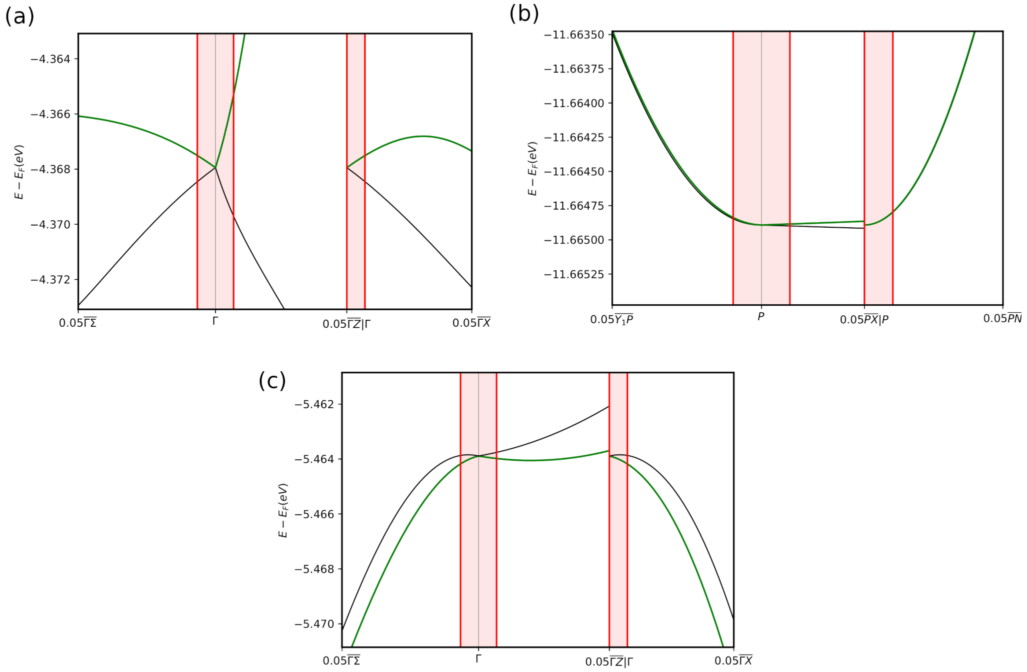


FIG. 6. Electronic band dispersion near the high-symmetry points of the selected bands used to illustrate the spin texture of $Ta_2Se_8I$. Vertical red lines delimit the radius of the sphere along the corresponding high-symmetry direction. Panel (a) shows band $n = 97$ (in green) which corresponds to the spin texture with linear momentum dependence illustrated in Fig. 1(d) of the main text. Panel (b) shows the band $n = 65$ used to compute the spin texture with quadratic momentum dependence illustrated in Fig. 2(a) of the main text. Panel (c) shows band $n = 72$ that correspond the spin texture with cubic momentum dependence shown in Fig. 3(c) in the main text.

### 4. $TaSi_2$

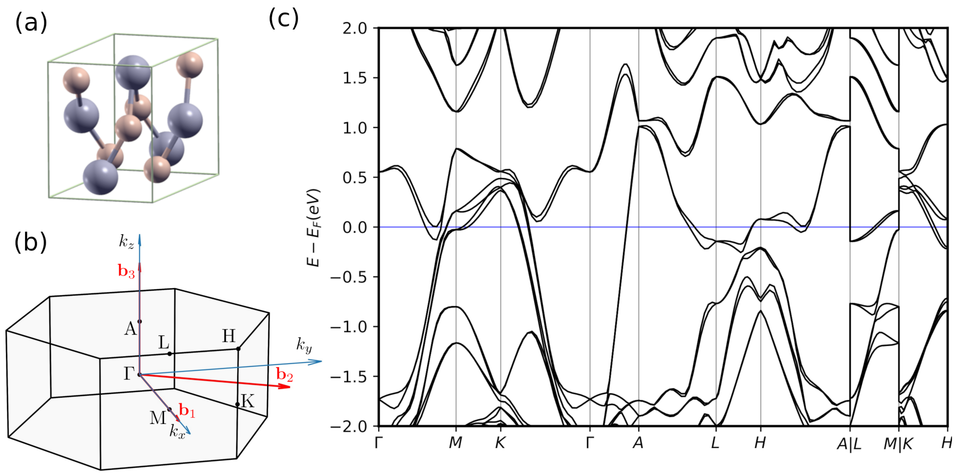


FIG. 7. (a) Crystal structure, (b) Brillouin zone with the high-symmetry points and reciprocal lattice vectors indicated, and (c) the calculated band structure of $TaSi_2$ plotted along the high-symmetry lines.

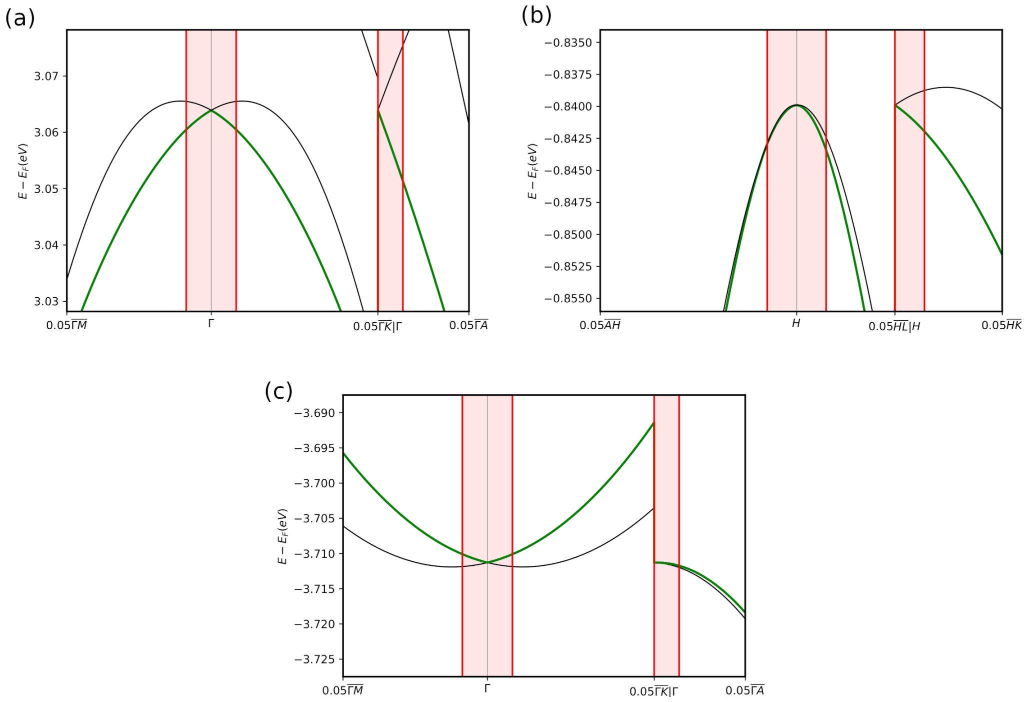


FIG. 8. Electronic band dispersion near the high-symmetry points of the selected bands used to illustrate the spin texture of $TaSi_2$. Vertical red lines delimit the radius of the sphere along the corresponding high-symmetry direction. Panel (a) shows band $n = 66$ (in green) which corresponds to the spin texture with linear momentum dependence illustrated in Fig. 1(e) of the main text. Panel (b) shows band $n = 56$ used to compute the spin texture with quadratic momentum dependence illustrated in Fig. 2(b) of the main text. Panel (c) shows band $n = 47$ that correspond the spin texture with cubic momentum dependence shown in Fig. 3(d) in the main text.

### 5. CoSi

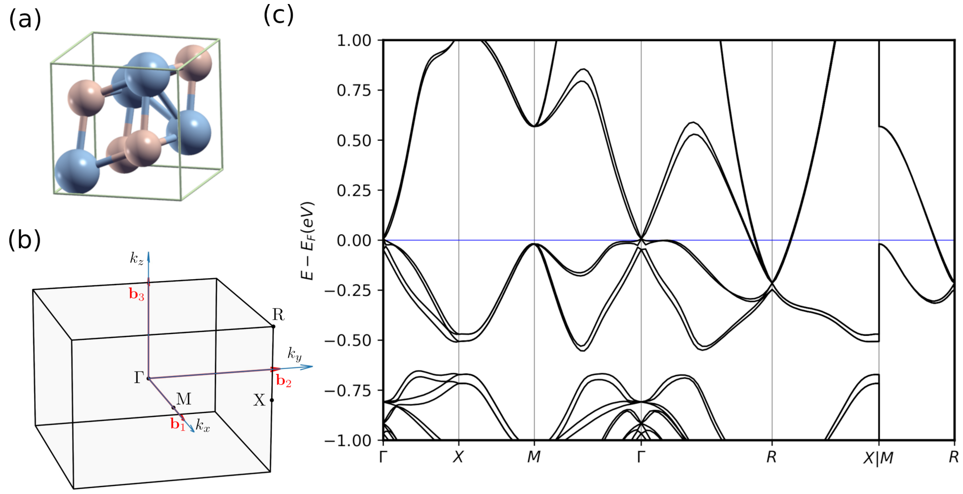


FIG. 9. (a) Crystal structure, (b) Brillouin zone with the high-symmetry points and reciprocal lattice vectors indicated, and (c) the calculated band structure of CoSi plotted along the high-symmetry lines.

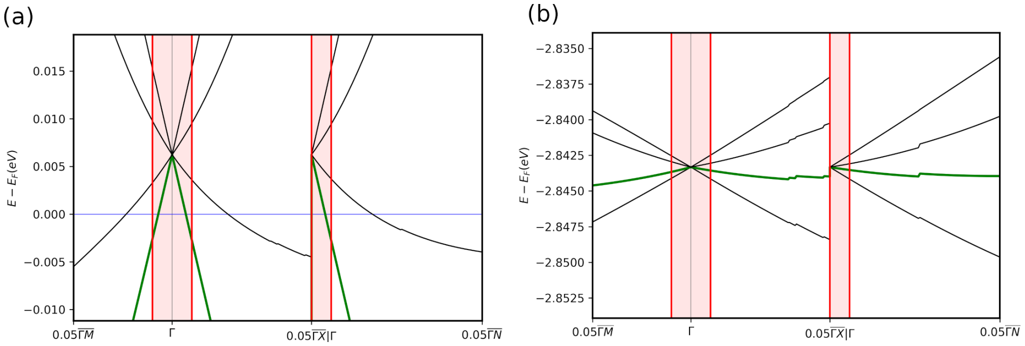


FIG. 10. Electronic band dispersion near the high-symmetry points of the selected bands used to illustrate the spin texture of CoSi. Vertical red lines delimit the radius of the sphere along the corresponding high-symmetry direction. Panel (a) shows band $n = 82$ (in green) which corresponds to the spin texture with linear momentum dependence illustrated in Fig. 1(a) of the main text. Panel (b) shows band $n = 59$ used to compute the spin texture with cubic momentum dependence illustrated in Fig. 3(e) of the main text.

*6.* $Ag_3AuTe_2$

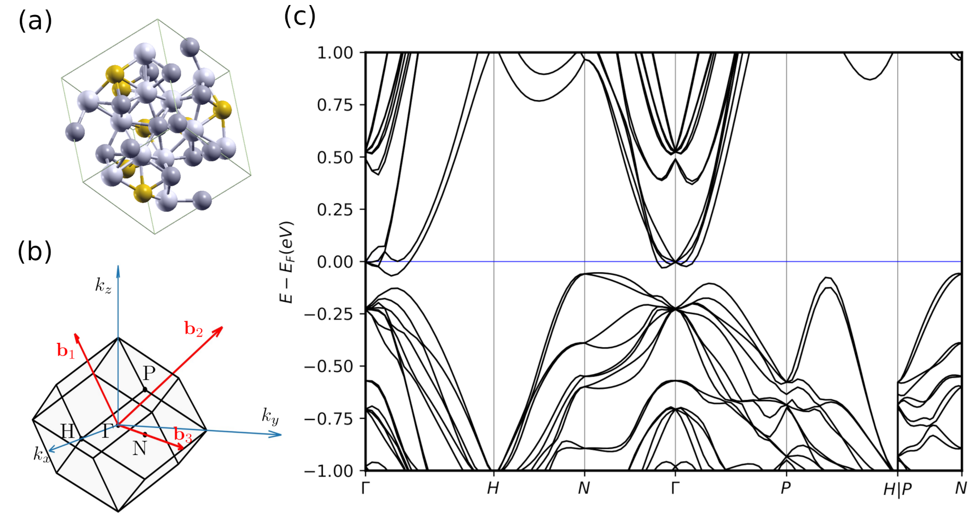


FIG. 11. (a) Crystal structure, (b) Brillouin zone with the high-symmetry points and reciprocal lattice vectors indicated, and (c) the calculated band structure of $Ag_3AuTe_2$ plotted along the high-symmetry lines.

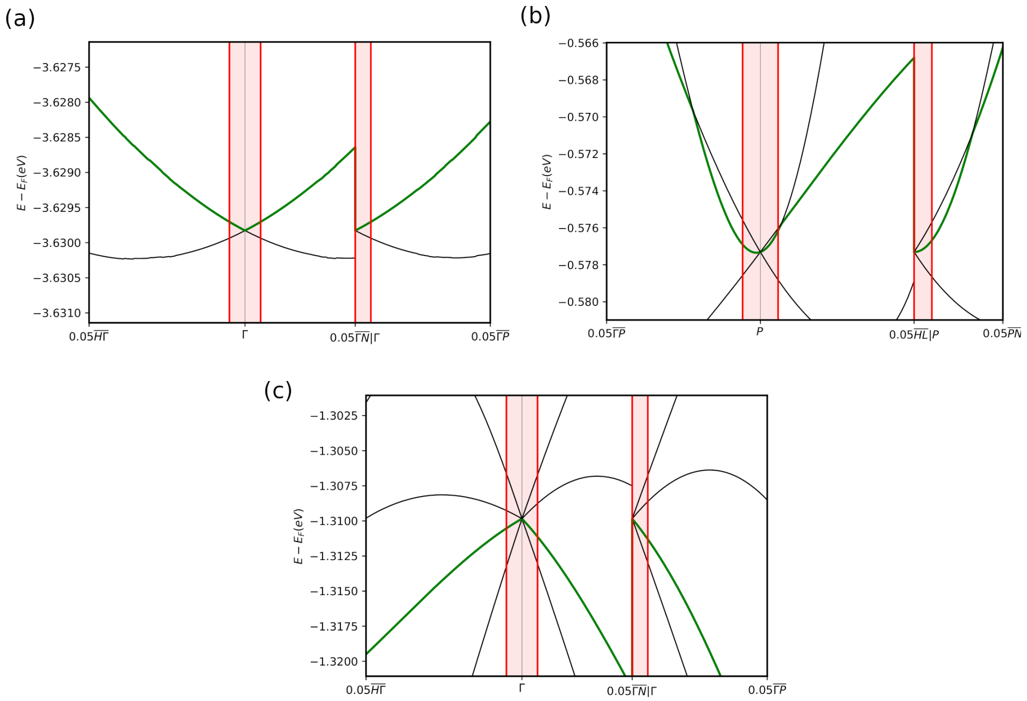


FIG. 12. Electronic band dispersion near the high-symmetry points of the selected bands used to illustrate the spin texture of $Ag_3AuTe_2$. Vertical red lines delimit the radius of the sphere along the corresponding high-symmetry direction. Panel (a) shows band $n = 153$ (in green) which corresponds to the spin texture with linear momentum dependence illustrated in Fig. 1(b) of the main text. Panel (b) shows band $n = 222$ used to compute the spin texture with quadratic momentum dependence illustrated in Fig. 2(c) of the main text. Panel (c) shows band $n = 203$ that correspond the spin texture with cubic momentum dependence shown in Fig. 3(f) in the main text.

## IV. RELATION BETWEEN THE VECTOR FIELDS AT NON-EQUIVALENT POINTS OF A GIVEN STAR

The star of a wavevector $\mathbf{k}_0$ is the set of non-equivalent points in the Brillouin zone, *i.e.* those points that are not related by a vector of the reciprocal lattice $\mathbf{G}$, that can be obtained by acting on $\mathbf{k}_0$ with the symmetry operations of the point group $\mathcal{G}$ that give rise to the space group of the corresponding crystal. The point group of $\mathbf{k}_0$, and of any non-equivalent point of the star, is $\mathcal{G}_{\mathbf{k}_0}$, a subgroup of the point group $\mathcal{G}$ of the space group ($\mathcal{G}_{\mathbf{k}_0} \subseteq \mathcal{G}$). Accordingly, the spin texture or any other vector field in momentum space around any non-equivalent point of the star of $\mathbf{k}_0$ is given by the Taylor expansion that satisfies point group symmetry $\mathcal{G}_{\mathbf{k}_0}$. The Taylor expansion coefficients are different for each of the non-equivalent points of the star of $\mathbf{k}_0$ However, these coefficients are related by $\mathcal{Q}_{\mathbf{k}_0} = \mathcal{G} - \mathcal{G}_{\mathbf{k}_0}$, complementary set of symmetry operation that are present in the point group $\mathcal{G}$ of the space group of the crystal but not present in $\mathcal{G}_{\mathbf{k}_0}$.

Therefore, the spin texture around high-symmetry points of the Brillouin zone whose point group is a subgroup of the point group of the space group can present simplifications in the general form of the vector field given by Table I of the main text. Here, we illustrate this simplification of the spin texture around the P point in $Ta_2Se_8I$. This material belongs to the space group $I422$ (No. 97) that contains the $D_4$ point group. According to the double-value representation tables in Ref. 12, the high-symmetry point $P$ have a point group symmetry $D_2$, and the star of $P$ contains two non-equivalent points $P$ and $P'$ as shown in Fig. 13.

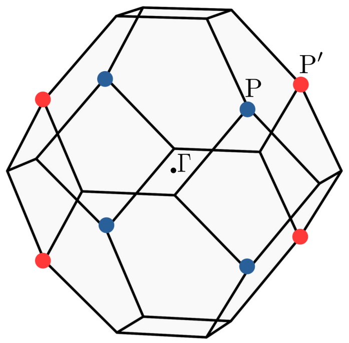


FIG. 13. Brillouin zone of $Ta_2Se_8I$ with non-equivalent points $P$ and $P'$.


[1] P. Giannozzi, S. Baroni, N. Bonini, M. Calandra, R. Car, C. Cavazzoni, D. Ceresoli, G. L. Chiarotti, M. Cococcioni, I. Dabo, *et al.*, Quantum espresso: a modular and open-source software project for quantum simulations of materials, J. Phys.: Condens. Matter **21**, 395502 (2009).

[2] J. P. Perdew, K. Burke, and M. Ernzerhof, Generalized gradient approximation made simple, Phys. Rev. Lett. **77**, 3865 (1996).

[3] A. Dal Corso, Pseudopotentials periodic table: From H to Pu, Comput. Mater. Sci. **95**, 337 (2014).

[4] D. R. Hamann, Optimized norm-conserving vanderbilt pseudopotentials, Phys. Rev. B **88**, 085117 (2013).

[5] M. Schlipf and F. Gygi, Optimization algorithm for the generation of oncv pseudopotentials, Comput. Phys. Commun. **196**, 36 (2015).

[6] S. Gražulis, D. Chateigner, R. T. Downs, A. F. T. Yokochi, M. Quirós, L. Lutterotti, E. Manakova, J. Butkus, P. Moeck, and A. Le Bail, Crystallography Open Database – an open-access collection of crystal structures, J. Appl. Crystallogr. **42**, 726 (2009).

[7] S. Gražulis, A. Daškevič, A. Merkys, D. Chateigner, L. Lutterotti, M. Quirós, N. R. Serebryanaya, P. Moeck, R. T. Downs, and A. Le Bail, Crystallography open database (cod): an open-access collection of crystal structures and platform for world-wide collaboration, Nucleic Acids Res. **40**, D420 (2012).

[8] A. Vaitkus, A. Merkys, and S. Gražulis, Validation of the Crystallography Open Database using the Crystallographic Information Framework, Journal of Applied Crystallography **54**, 661 (2021).

[9] D. Zagorac, H. Müller, S. Ruehl, J. Zagorac, and S. Rehme, Recent developments in the Inorganic Crystal Structure Database: theoretical crystal structure data and related features, J. Appl. Crystallogr. **52**, 918 (2019).

[10] T. Björkman, Cif2cell: Generating geometries for electronic structure programs, Comput. Phys. Commun. **182**, 1183 (2011).

[11] N. Marzari, D. Vanderbilt, A. De Vita, and M. C. Payne, Thermal contraction and disordering of the al(110) surface, Phys. Rev. Lett. **82**, 3296 (1999).

[12] C. Bradley and A. Cracknell, *The Mathematical Theory of Symmetry in Solids: Representation Theory for Point Groups and Space Groups*, EBSCO ebook academic collection (OUP Oxford, 2010).
